# Supplementary material for: CLiMB: A Continual Learning Benchmark for Vision-and-Language Tasks
Source: arXiv:2206.09059 source file (2022-11-24)
Supplement: Supplementary file 1 [file uniter-forgetting.tex]

\begin{table}[ht]
    \setlength{\aboverulesep}{0pt}
    \setlength{\belowrulesep}{0pt}
    \centering
    \begin{small}
\begin{tabular}{lrr}
    \multicolumn{3}{c}{CL Algorithm: Sequential Fine-tuning} \\
    \toprule
    %\multicolumn{7}{c}{Comparison of Algorithms (Fixed Task Order, Encoder=ViLT)}\\
    %\toprule
    \multirow{2}{*}{\backslashbox{Checkpoint}{Evaluated on}} & \multicolumn{1}{c}{Task 1} & \multicolumn{1}{c}{Task 2} \\
    &  \multicolumn{1}{c}{VQAv2} & \multicolumn{1}{c}{NLVR2} \\
    \midrule
    After training on that task & [70.01]	& [74.61] \\
    \midrule
    Task 2: NLVR2  &  \transfer{6.25}{65.64}	& - \\
    Task 3: SNLI-VE &   \transfer{32.20}{47.46} & \transfer{50.00}{62.30} \\
    \bottomrule
    \\
    \multicolumn{3}{c}{CL Algorithm: Experience Replay} \\
    \toprule
    %\multicolumn{7}{c}{Comparison of Algorithms (Fixed Task Order, Encoder=ViLT)}\\
    %\toprule
    \multirow{2}{*}{\backslashbox{Checkpoint}{Evaluated on}} & \multicolumn{1}{c}{Task 1} & \multicolumn{1}{c}{Task 2} \\
    &  \multicolumn{1}{c}{VQAv2} & \multicolumn{1}{c}{NLVR2} \\
    \midrule
    After training on that task & [69.90]	& [75.45] \\
    \midrule
    Task 2: NLVR2  &  \transfer{2.83}{67.92}	& - \\
    Task 3: SNLI-VE &   \transfer{6.61}{65.28} & \transfer{24.76}{69.15} \\
    \bottomrule
    \end{tabular}
    \end{small}
    \caption{Full numbers for forgetting transfer $\forgetting{j}{i}$ of previously seen tasks for Sequential Fine-tuning and Experience Replay, using UNITER as the pre-trained vision-language encoder. We also show the  transfer score $[S_\algorithm^{j \leftarrow i}]$ when evaluated on that task after training on future task $i$. The first row contains task score $[S_\algorithm^j]$ after originally training on $j^{th}$ task.
    }
\label{tab:uniter-forgetting}
\end{table}
